# Supplementary material for: Implications on Feature Detection when using the Benefit-Cost Ratio
Source: arXiv:2008.05163 ancillary file (2020-08-15)
Supplement: Supplementary file 1 [file Additional_file_2.pdf]

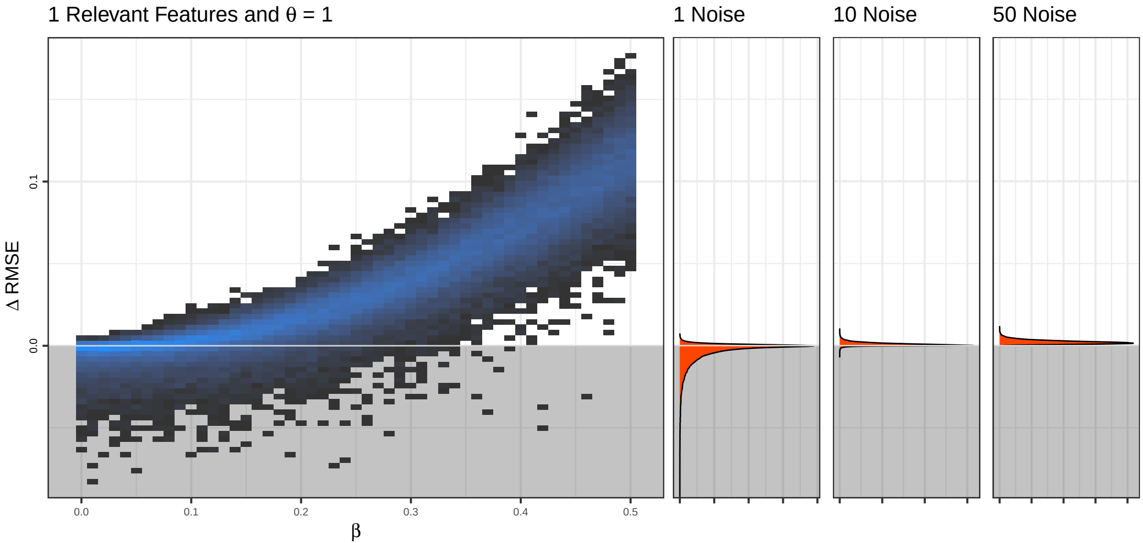

1 Relevant Features and θ = 1
1 Noise
10 Noise
50 Noise
Δ RMSE
0.1
0.0
0.0
0.1
0.2
0.3
0.4
0.5
β

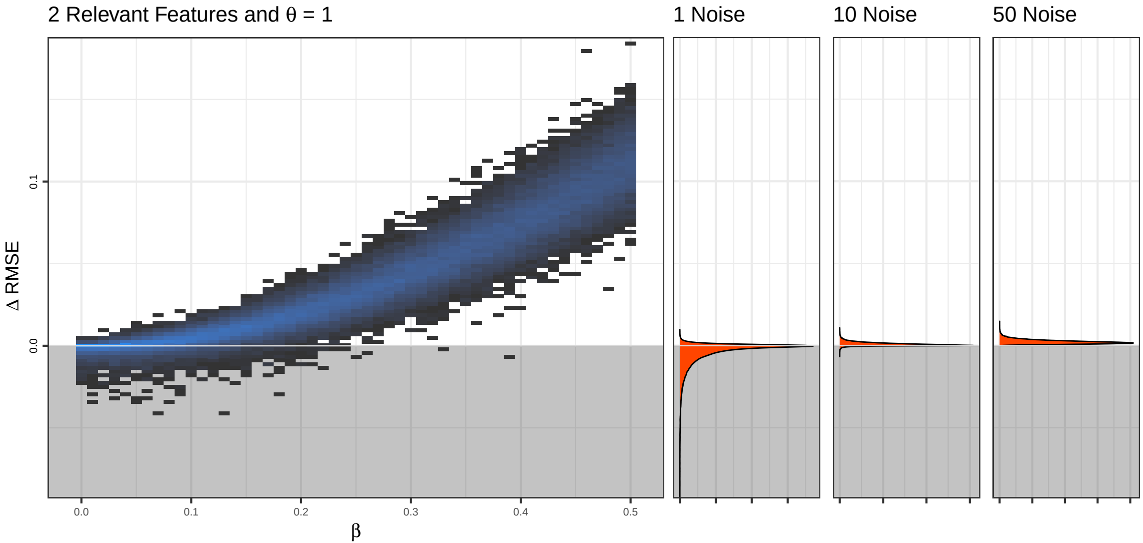

2 Relevant Features and θ = 1
1 Noise
10 Noise
50 Noise
Δ RMSE
0.1
0.0
0.0
0.1
0.2
0.3
0.4
0.5
β

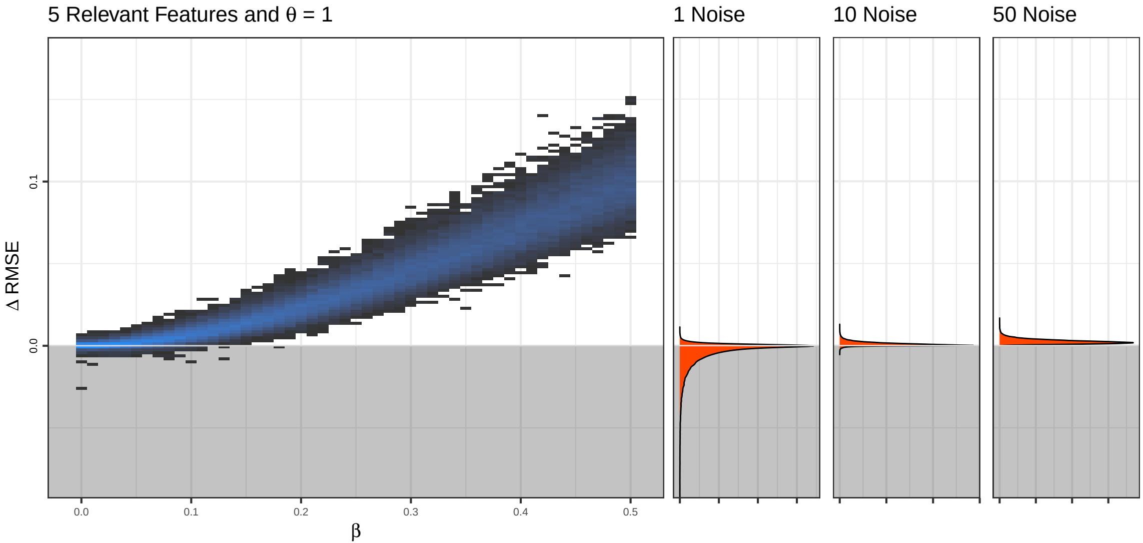

5 Relevant Features and θ = 1
1 Noise
10 Noise
50 Noise
Δ RMSE
0.1
0.0
0.0
0.1
0.2
0.3
0.4
0.5
β

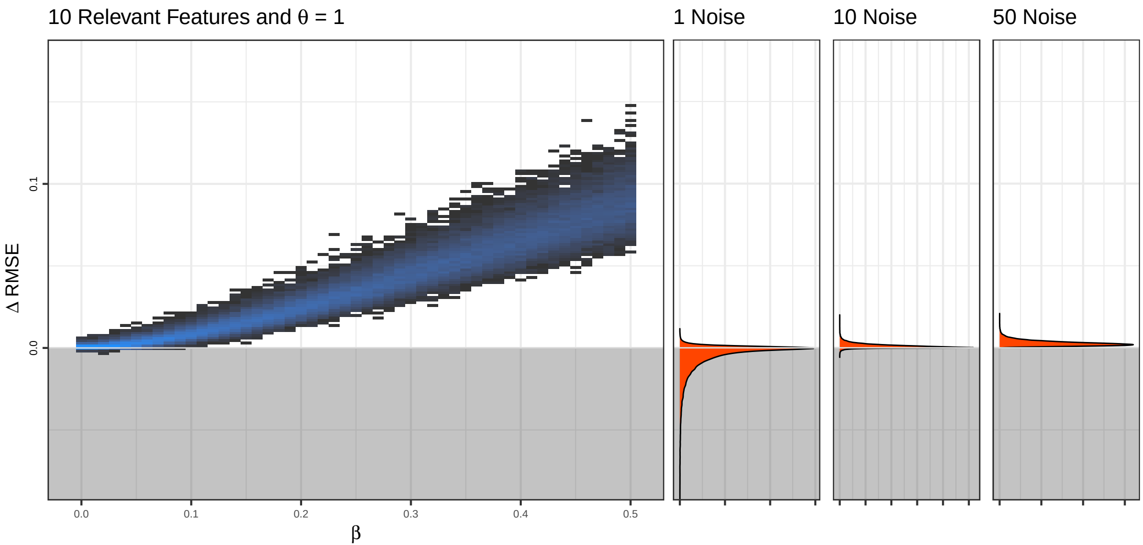
10 Relevant Features and θ = 1
1 Noise
10 Noise
50 Noise
Δ RMSE
0.1
0.0
0.0
0.1
0.2
0.3
0.4
0.5
β

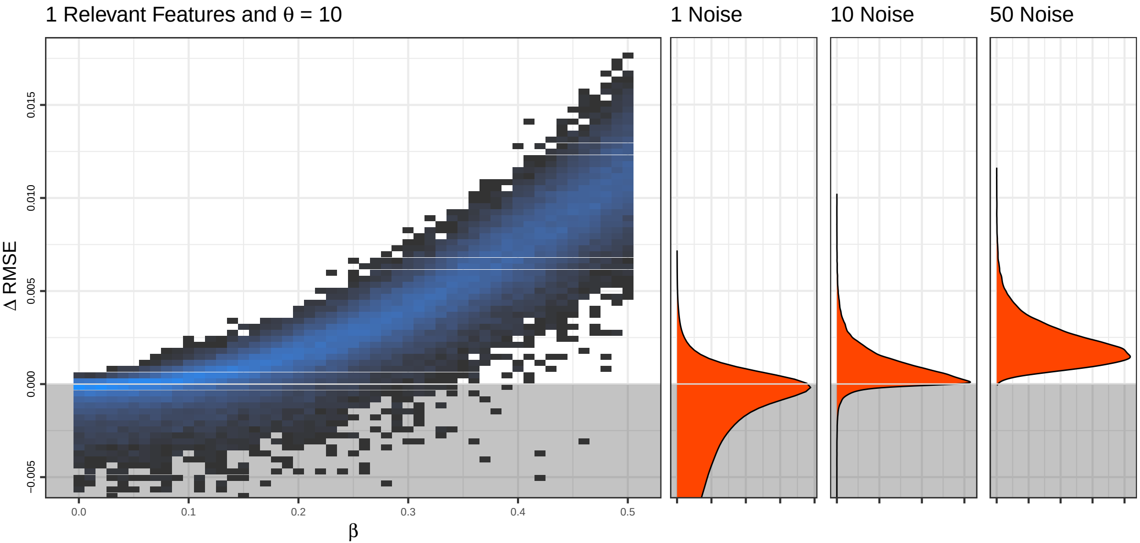

1 Relevant Features and θ = 10
1 Noise
10 Noise
50 Noise
Δ RMSE
0.015
0.010
0.005
0.000
−0.005
0.0
0.1
0.2
0.3
0.4
0.5
β

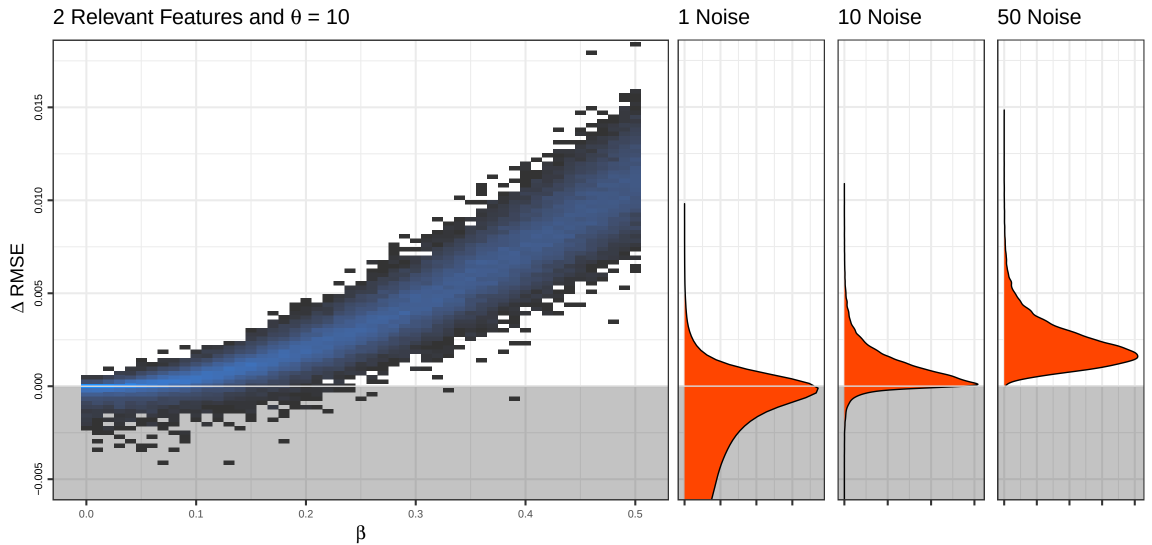
2 Relevant Features and θ = 10
1 Noise
10 Noise
50 Noise
Δ RMSE
0.015
0.010
0.005
0.000
−0.005
0.0
0.1
0.2
0.3
0.4
0.5
β

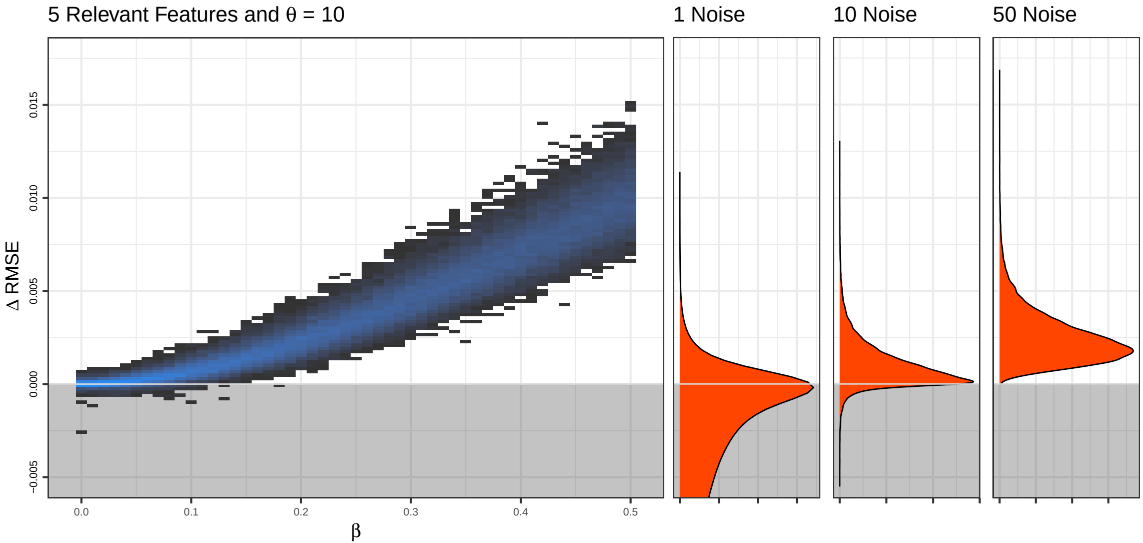

5 Relevant Features and θ = 10
1 Noise
10 Noise
50 Noise
Δ RMSE
0.015
0.010
0.005
0.000
−0.005
0.0
0.1
0.2
0.3
0.4
0.5
β

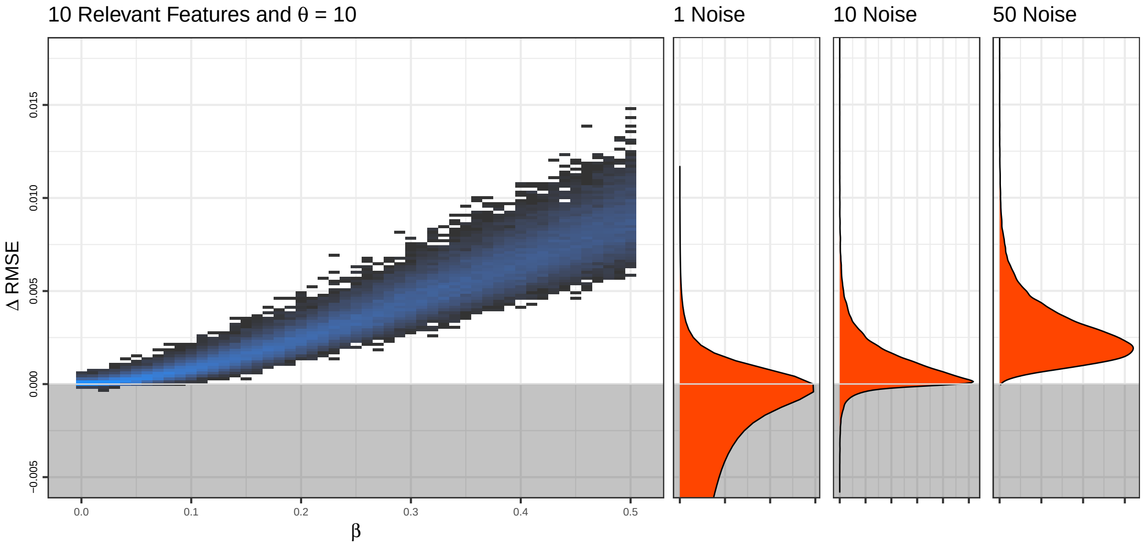
10 Relevant Features and θ = 10
1 Noise
10 Noise
50 Noise
Δ RMSE
−0.005
0.000
0.005
0.010
0.015
0.0
0.1
0.2
0.3
0.4
0.5
β

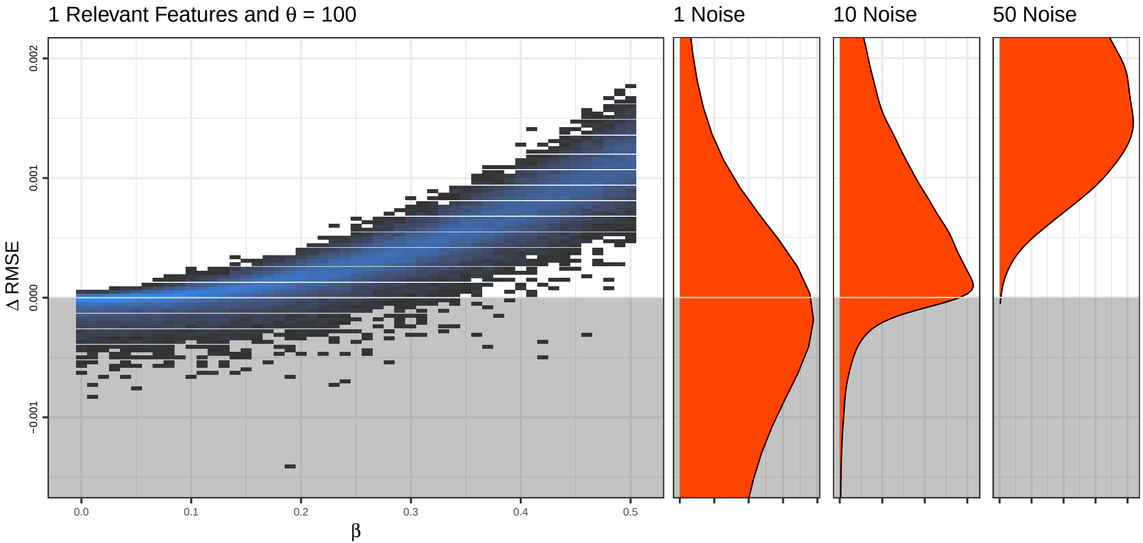

1 Relevant Features and θ = 100
1 Noise
10 Noise
50 Noise
Δ RMSE
0.002
0.001
0.000
−0.001
0.0
0.1
0.2
0.3
0.4
0.5
β

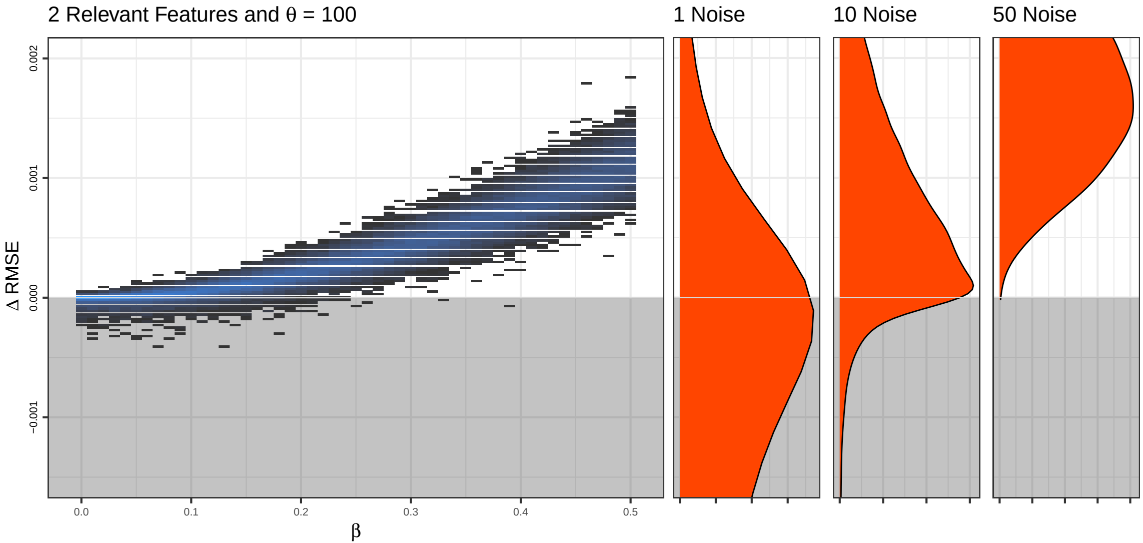

2 Relevant Features and θ = 100
1 Noise
10 Noise
50 Noise
Δ RMSE
0.002
0.001
0.000
−0.001
0.0
0.1
0.2
0.3
0.4
0.5
β

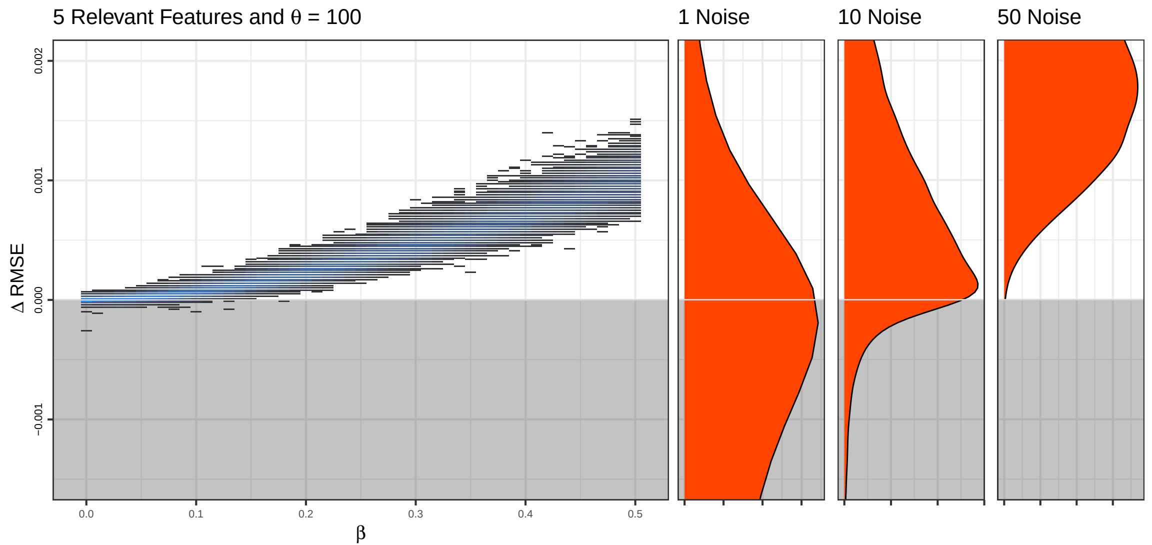

5 Relevant Features and θ = 100
1 Noise
10 Noise
50 Noise
Δ RMSE
0.002
0.001
0.000
−0.001
0.0
0.1
0.2
0.3
0.4
0.5
β

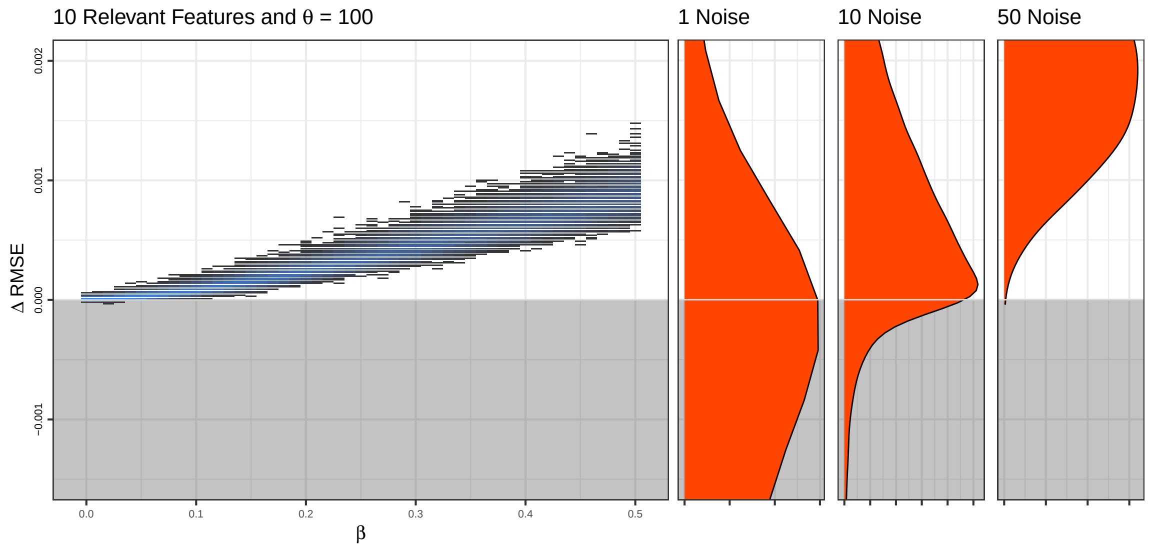

10 Relevant Features and θ = 100
1 Noise
10 Noise
50 Noise
Δ RMSE
0.002
0.001
0.000
−0.001
0.0
0.1
0.2
0.3
0.4
0.5
β

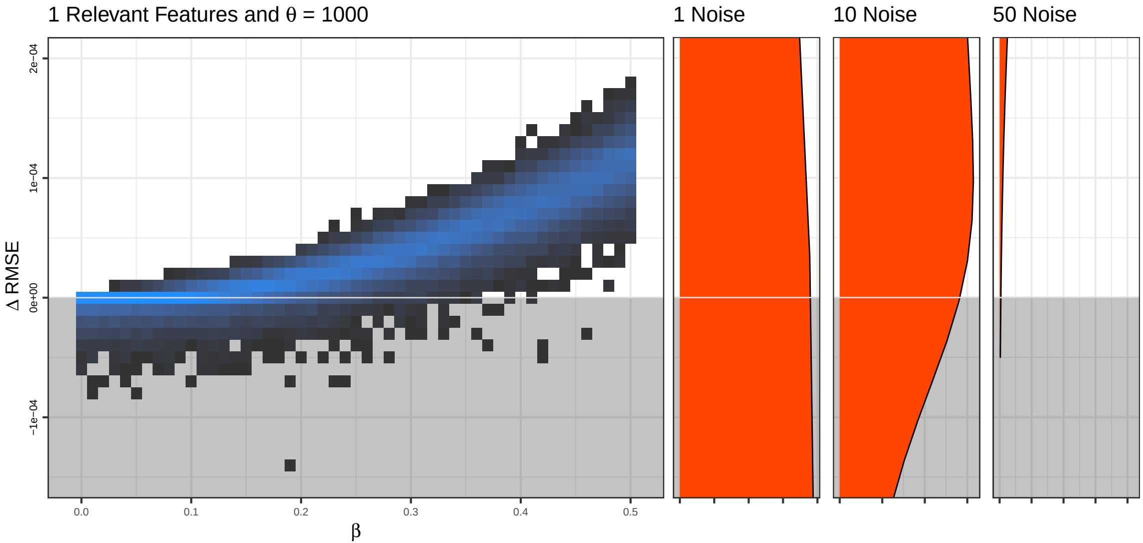
1 Relevant Features and θ = 1000
1 Noise
10 Noise
50 Noise
Δ RMSE
2e−04
1e−04
0e+00
−1e−04
0.0
0.1
0.2
0.3
0.4
0.5
β

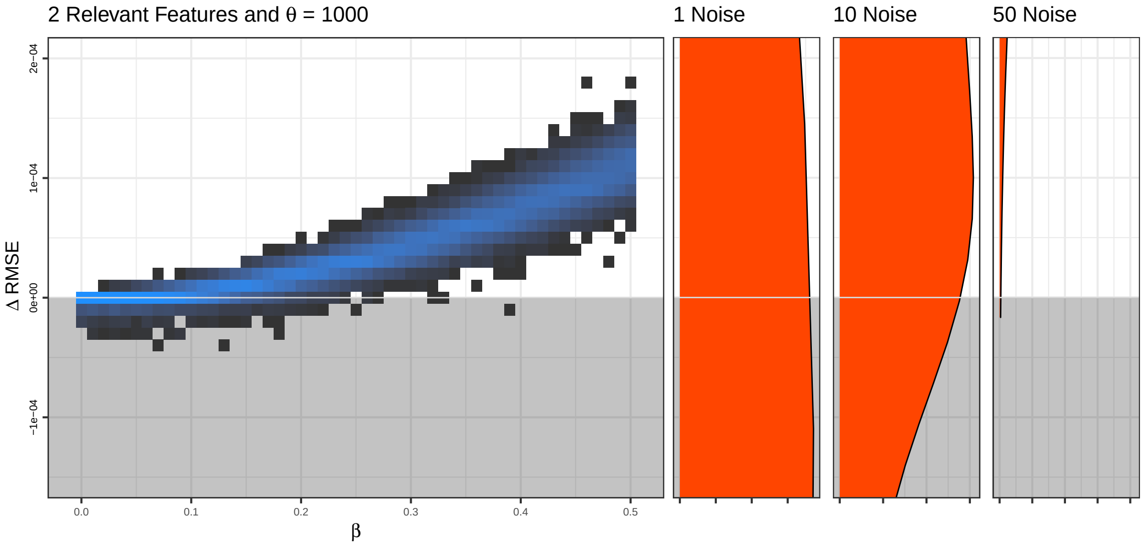

2 Relevant Features and θ = 1000
1 Noise
10 Noise
50 Noise
2e−04
1e−04
0e+00
−1e−04
Δ RMSE
0.0
0.1
0.2
0.3
0.4
0.5
β

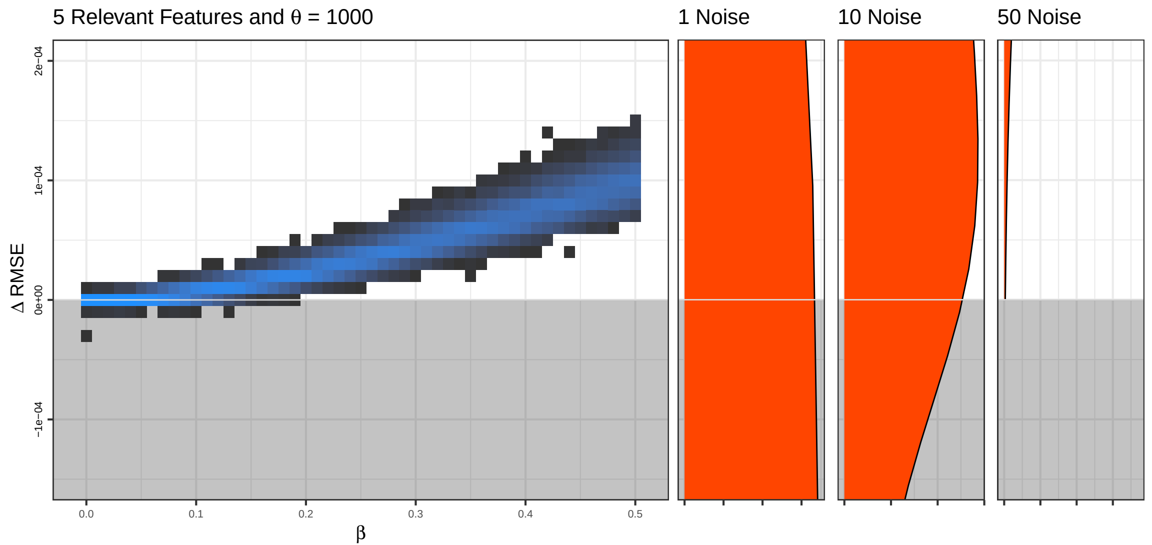

5 Relevant Features and θ = 1000
1 Noise
10 Noise
50 Noise
Δ RMSE
2e−04
1e−04
0e+00
−1e−04
0.0
0.1
0.2
0.3
0.4
0.5
β

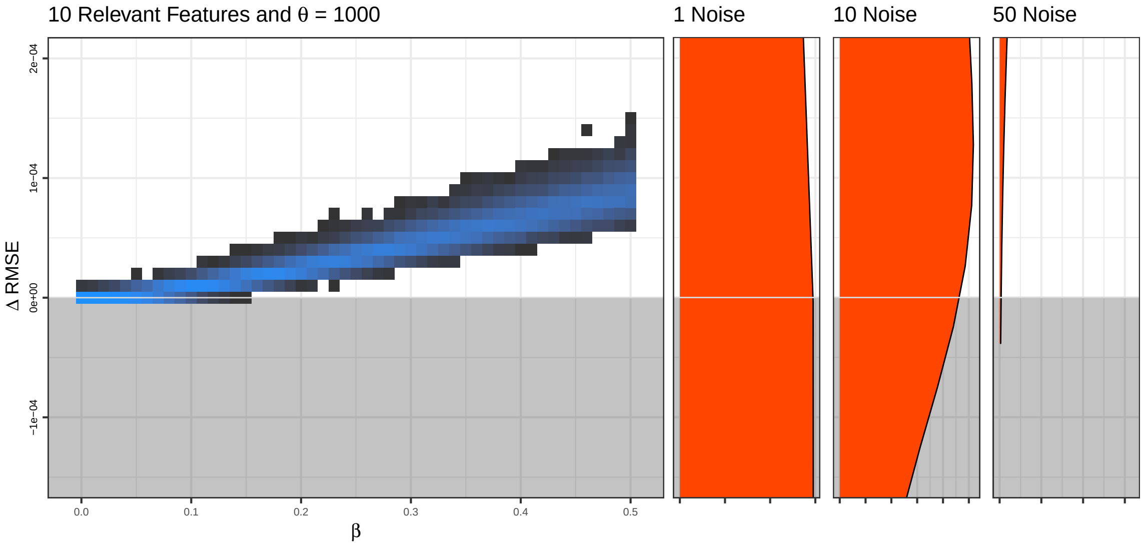

10 Relevant Features and θ = 1000
1 Noise
10 Noise
50 Noise
2e−04
1e−04
0e+00
−1e−04
Δ RMSE
0.0
0.1
0.2
0.3
0.4
0.5
β
