# Supplementary material for: Implications on Feature Detection when using the Benefit-Cost Ratio
Source: arXiv:2008.05163 ancillary file (2020-08-15)

# Scaling Analysis (1 Relevant Feature)

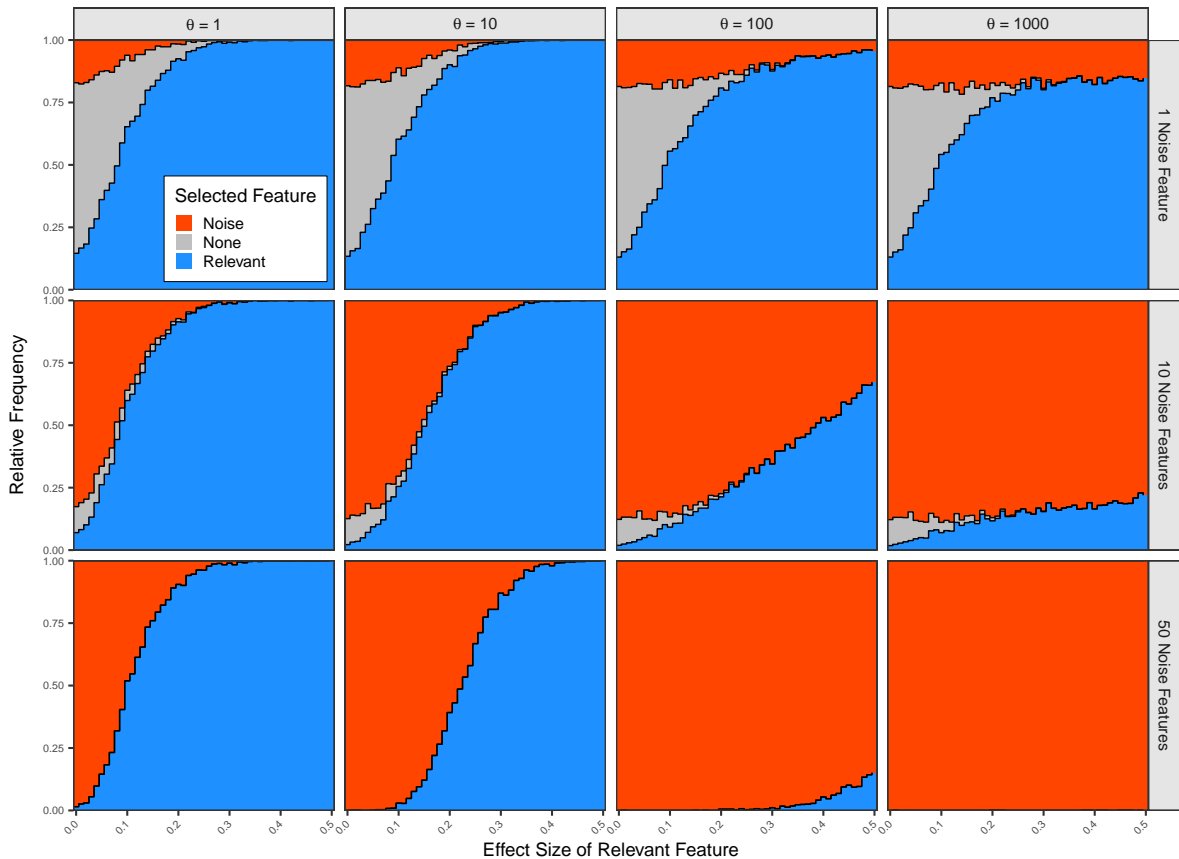

## Scaling Analysis (2 Relevant Features)

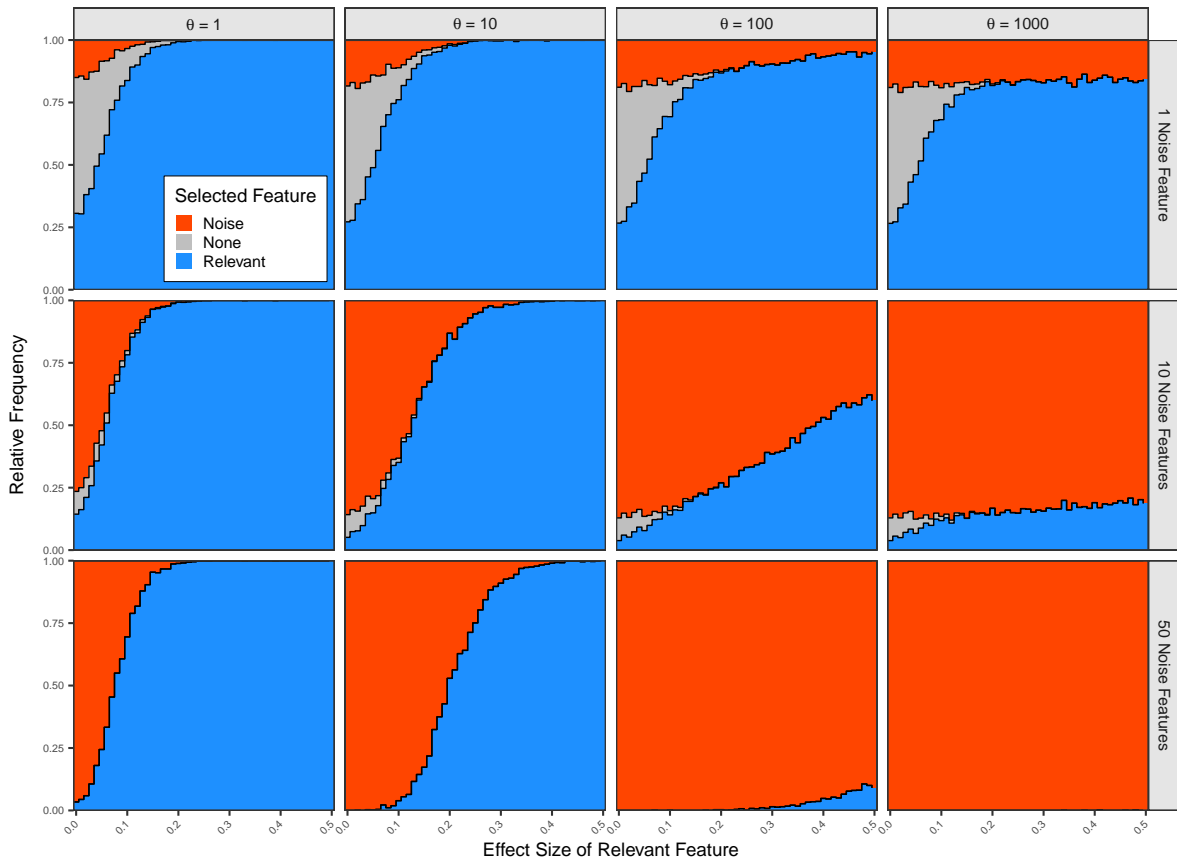

# Scaling Analysis (5 Relevant Features)

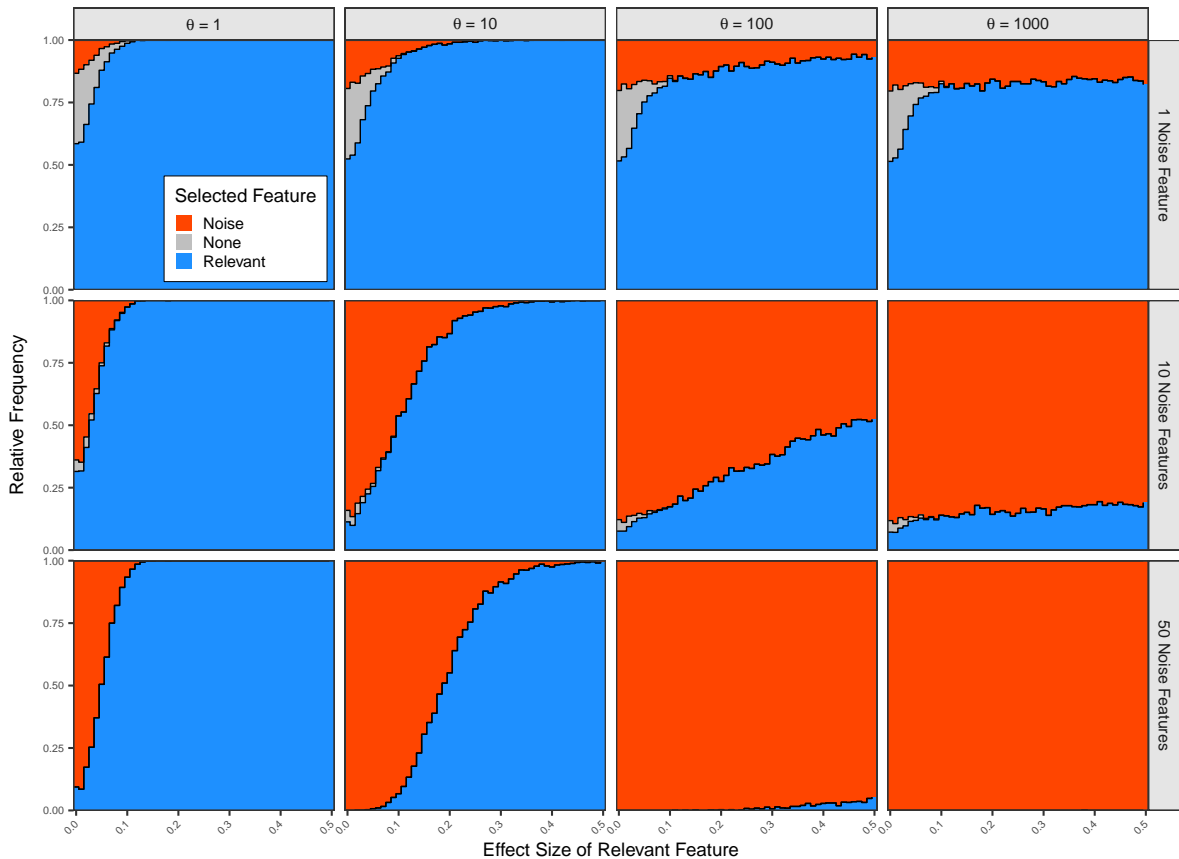

# Scaling Analysis (10 Relevant Features)

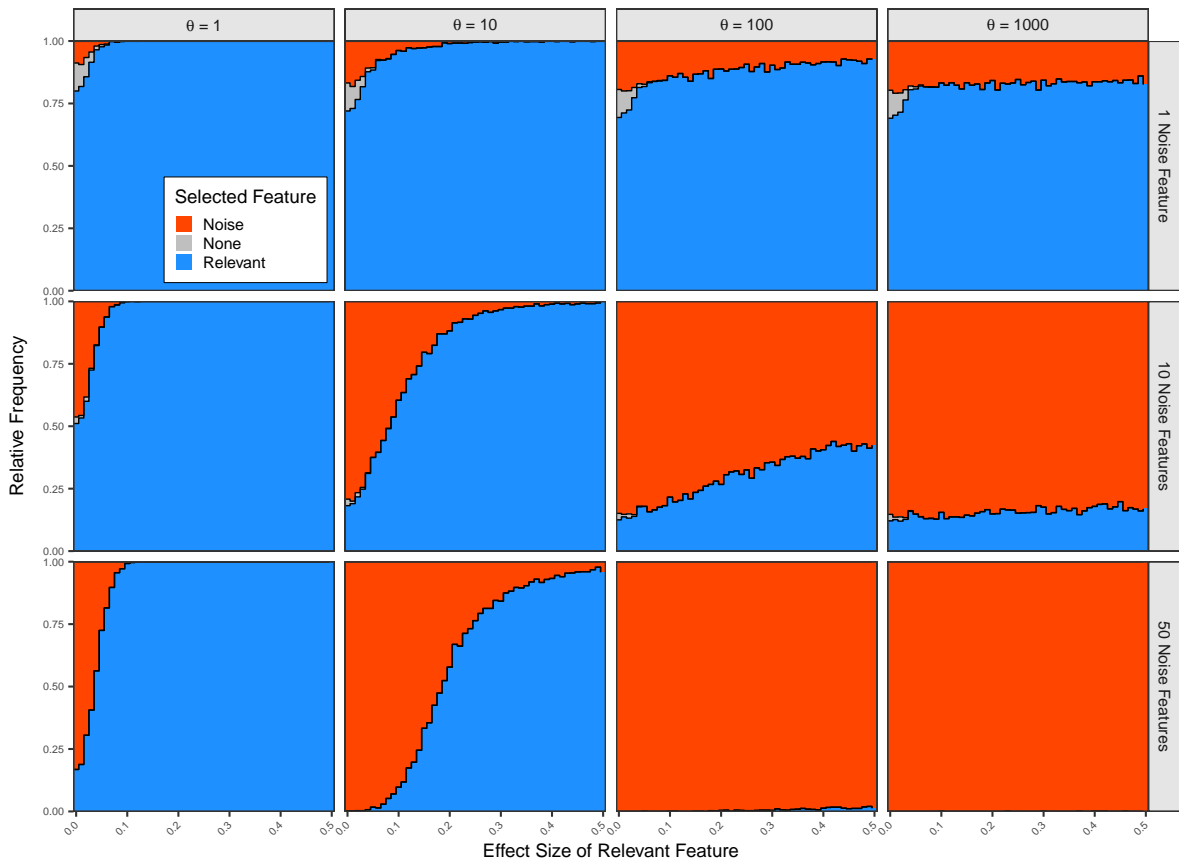

Supplement: Supplementary file 2 [file Additional_file_1.pdf]
